# Supplementary material for: Experiments and a User Study for Hierarchical Drawings of Graphs
Source: arXiv:2209.04522 source file (2022-09-09)
Supplement: Supplementary file 1 [file appendix.tex]

\appendix
\section{Appendix}
